# Supplementary material for: Attention, Please! Revisiting Attentive Probing Through the Lens of Efficiency
Source: arXiv:2506.10178 source file (2026-02-18)
Supplement: Supplementary file 1 [file imagenet_val_attmaps_q8_supp.tex]

\setlength{\tabcolsep}{1.2pt}
\newcommand{\sz}{1.65cm}

% A small helper: label above, image below (centered), fixed width \sz
\newcommand{\imcell}[2]{%
  \begin{minipage}[t]{\sz}
    \centering
    \if\relax\detokenize{#1}\relax\else $#1$\\[2pt]\fi
    \includegraphics[width=\sz,height=\sz]{#2}%
  \end{minipage}%
}

\begin{subfigure}{\textwidth}
  \centering
  % Replace paths below with your second set (examples shown as *_8 ... *_15)
  \imcell{}{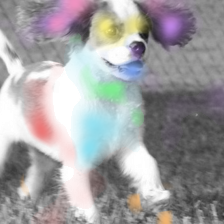}\hspace{1.2pt}
  \imcell{}{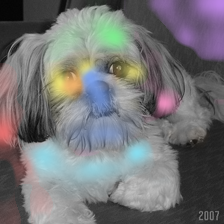}\hspace{1.2pt}
  \imcell{}{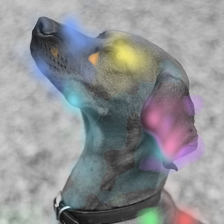}\hspace{1.2pt}
  \imcell{}{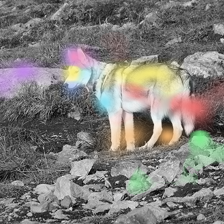}\hspace{1.2pt}
  \imcell{}{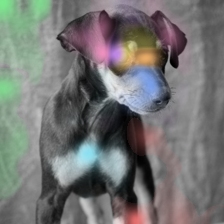}\hspace{1.2pt}
  \imcell{}{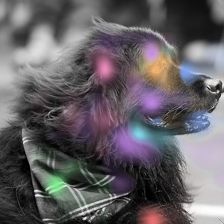}\hspace{1.2pt}
  \imcell{}{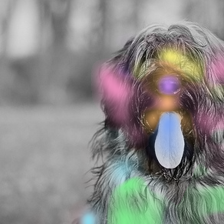}\hspace{1.2pt}
  \imcell{}{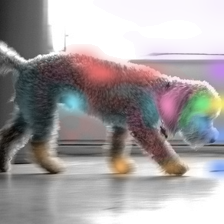}
  
\end{subfigure}
